# Supplementary material for: Sub-Character Tokenization for Chinese Pretrained Language Models
Source: arXiv:2106.00400 source file (2023-02-14)
Supplement: Supplementary file 1 [file appendix.tex]

\subsection{What is \shuowen-\jiezi?}
\label{app:shuowenjiezi}

\shuowen-\jiezi~ (`说文解字') is an ancient Chinese dictionary from the Han dynasty. 
It was the first dictionary to analyze the structure of Chinese characters and to give the rationale behind them, and also the first dictionary to use Chinese radicals to organise the sections.

The literal meaning of \shuowen~ and \jiezi~ correspond nicely to the core intuitive behind our pronunciation- and glyph-based tokenizers. We name our methods this name to pay tribute to the ancient wisdom of our ancestors. 

\subsection{Input Methods}
\label{app:inputmethod}

Current Chinese input methods for computers can be categorized into pronunciation-based and glyph-based. Both methods encode each Chinese character into a sequence of units from a smaller set of alphabet (e.g. the Latin alphabet), but differ in what the units represent. In pronunciation-based input methods, each unit usually represents a phoneme, while in glyph-based methods, one unit or a group of units generally represent a radical or stoke composition. Chinese characters have a standardized stroke order, which can be taken into account by glyph-based methods. In almost all commonly used input methods, there exists different characters that encode into the same sequence, in which case, the solution is usually to list all matching characters and let the user select the correct one. We briefly introduce each input method used in the paper below.

\noindent \textbf{Cangjie} (`仓颉') and \textbf{Wubi} (`五笔') are two similar glyph-based input methods. They map keys on the QWERTY keyboard to fundamental radicals or combination of strokes that are combined to represent the shape of entire characters. They sometimes disregard stroke order in favor of combinations that visually more similar to the character. The main difference between them is the key mapping and the rules on how to break down characters into fundamental components.

\noindent \textbf{Zhengma} (`郑码'), a glyph-based method, is similar to Cangjie and Wubi. It maps each Latin letter to fundamental radicals, which are combined into entire characters. But Zhengma differs from Cangjie and Wubi in that it strictly follows stroke order.

\noindent \textbf{Stroke} (`笔画'), a glyph-based method, more commonly used in mobile phones or numerical keypads, maps five keys to five basic types of strokes. The user pressed the corresponding keys according to characters' stroke order. 

\noindent \textbf{Pinyin} (`拼音') input method, a pronunciation-based input method, is the most widely used input method among Chinese speakers. It is based on the Hanyu Pinyin (`汉语拼音', meaning Chinese Sound-Spelling) romanization system for Chinese. Each Chinese monophthong is mapping to one or two Latin alphabet. 

\noindent \textbf{Zhuyin} (`注音') input method, a pronunciation-based input method, is the most common input method in the Taiwan province of China. It is based on the Zhuyin phonetic transcription system, which consists 37 characters that represent each Chinese phoneme. Note that while both Pinyin and Zhuyin input methods disregard tones as input methods on electonic devices, we do keep the tones during encoding in our tokenizers.
